# Supplementary material for: Decoherence and Quantum Error Correction for Quantum Computing and Communications
Source: arXiv:2202.08600 source file (2022-02-17)
Supplement: Supplementary file 1 [file sup-mat-pat.pdf]

# Supplementary information for Time-varying Quantum Channel Models for Superconducting Qubits

Josu Etxezarreta Martinez<sup>1,\*</sup>, Patricio Fuentes<sup>1</sup>, Pedro Crespo<sup>1</sup> and Javier Garcia-Frias<sup>2</sup>

Tecnun - University of Navarra<sup>1</sup>

University of Delaware<sup>2</sup>

*jetxezarreta@tecnun.es\**

June 22, 2021

## Supplementary Note 1: Proof for $\|\mathcal{N}_{\text{ADPTA}}(\gamma_1) - \mathcal{N}_{\text{ADPTA}}(\gamma_2)\|_\diamond = \|\mathcal{N}_{\text{ADCTA}}(\gamma_1) - \mathcal{N}_{\text{ADCTA}}(\gamma_2)\|_\diamond$

**Proposition 1.** The diamond norm distance between the Pauli twirl approximated channels (PTA) obtained from two amplitude damping channels (AD) of parameters  $\gamma_1$  and  $\gamma_2$  is the same as the diamond norm distance between the Clifford twirl approximated channels (CTA) obtained from the same AD channels:

$$\|\mathcal{N}_{\text{ADPTA}}(\gamma_1) - \mathcal{N}_{\text{ADPTA}}(\gamma_2)\|_\diamond = \|\mathcal{N}_{\text{ADCTA}}(\gamma_1) - \mathcal{N}_{\text{ADCTA}}(\gamma_2)\|_\diamond. \quad (1)$$

*Proof.* The PTA and CTA channels are Pauli channels [1]. The PTA channel for an AD channel with damping probability  $\gamma$  has the following probabilities for each of the Pauli matrices:

$$p_I = \frac{2 - \gamma + 2\sqrt{1 - \gamma}}{4}, p_x = p_y = \frac{\gamma}{4} \text{ and } p_z = \frac{2 - \gamma - 2\sqrt{1 - \gamma}}{4}.$$

The CTA channel is a depolarizing channel (as a special case of the Pauli channels), with the following probabilities:

$$r_I = \frac{2 - \gamma + 2\sqrt{1 - \gamma}}{4} \text{ and } r/3 = r_x = r_y = r_z = \frac{2 + \gamma - 2\sqrt{1 - \gamma}}{12}.$$

The diamond norm distance between Pauli channels has the closed-form expression [2]

$$\|\mathcal{N}_P^1 - \mathcal{N}_P^2\|_\diamond = \sum_k |p_k^1 - p_k^2|, \quad (2)$$

with  $k \in \{I, X, Y, Z\}$ . Knowing that the PTAs and CTAs are Pauli channels, we can write the diamond norm distances between them obtained from approximating two AD channels:

- (a)  $\|\mathcal{N}_{\text{ADPTA}}(\gamma_1) - \mathcal{N}_{\text{ADPTA}}(\gamma_2)\|_\diamond = |p_I^1 - p_I^2| + |p_x^1 - p_x^2| + |p_y^1 - p_y^2| + |p_z^1 - p_z^2|$
- (b)  $\|\mathcal{N}_{\text{ADCTA}}(\gamma_1) - \mathcal{N}_{\text{ADCTA}}(\gamma_2)\|_\diamond = |r_I^1 - r_I^2| + \sum_{l=x,y,z}^3 |r_l^1 - r_l^2| = |r_I^1 - r_I^2| + 3|r^1/3 - r^2/3|$

Note that  $p_I = r_I, \forall \gamma$ , so the contribution of the probabilities associated to non-identity components to the diamond norm distances must be compared. We start by expanding (b):

$$\begin{aligned} 3|r^1/3 - r^2/3| &= 3 \left| \frac{\gamma_1 - \gamma_2 + 2(\sqrt{1 - \gamma_2} - \sqrt{1 - \gamma_1})}{12} \right| \\ &= \frac{1}{4} |\gamma_1 - \gamma_2 + 2(\sqrt{1 - \gamma_2} - \sqrt{1 - \gamma_1})|. \end{aligned} \quad (3)$$

The results shown below for the terms  $\gamma_1 - \gamma_2$  and  $\sqrt{1 - \gamma_2} - \sqrt{1 - \gamma_1}$  that appear in equation (3) will be useful in what follows:

- $\gamma_1 - \gamma_2 > 0 \rightarrow \gamma_1 > \gamma_2 \rightarrow -\gamma_1 < -\gamma_2 \rightarrow 1 - \gamma_1 < 1 - \gamma_2 \rightarrow \sqrt{1 - \gamma_1} < \sqrt{1 - \gamma_2} \rightarrow \sqrt{1 - \gamma_2} - \sqrt{1 - \gamma_1} > 0.$
- $\gamma_1 - \gamma_2 < 0 \rightarrow \gamma_1 < \gamma_2 \rightarrow -\gamma_1 > -\gamma_2 \rightarrow 1 - \gamma_1 > 1 - \gamma_2 \rightarrow \sqrt{1 - \gamma_1} > \sqrt{1 - \gamma_2} \rightarrow \sqrt{1 - \gamma_2} - \sqrt{1 - \gamma_1} < 0.$
- $\gamma_1 - \gamma_2 = 0 \rightarrow \sqrt{1 - \gamma_2} - \sqrt{1 - \gamma_1} = 0.$

From these observations, it is easy to see that  $\gamma_1 - \gamma_2$  and  $\sqrt{1 - \gamma_2} - \sqrt{1 - \gamma_1}$  share the same sign  $\forall \gamma_1, \gamma_2$ . Thus, we can split the sum inside the absolute value of (3) into a sum of absolute values as

$$(3) = \frac{1}{4}|\gamma_1 - \gamma_2| + \frac{1}{2}|\sqrt{1 - \gamma_2} - \sqrt{1 - \gamma_1}|. \quad (4)$$

We continue by developing the non-identity part for the PTA as given in (a):

$$\begin{aligned} |p_x^1 - p_x^2| + |p_y^1 - p_y^2| + |p_z^1 - p_z^2| &= \frac{|\gamma_1 - \gamma_2|}{4} + \frac{|\gamma_1 - \gamma_2|}{4} \\ &\quad + \frac{|\gamma_2 - \gamma_1 + 2(\sqrt{1 - \gamma_2} - \sqrt{1 - \gamma_1})|}{4}. \end{aligned} \quad (5)$$

We follow the same reasoning as for the CTA by making use of the following expressions that  $\gamma_2 - \gamma_1$  and  $\sqrt{1 - \gamma_2} - \sqrt{1 - \gamma_1}$  fulfil. They are later added within the absolute value of their corresponding terms in the expression:

- $\gamma_2 - \gamma_1 > 0 \rightarrow \gamma_2 > \gamma_1 \rightarrow -\gamma_2 < -\gamma_1 \rightarrow 1 - \gamma_2 < 1 - \gamma_1 \rightarrow \sqrt{1 - \gamma_2} < \sqrt{1 - \gamma_1} \rightarrow \sqrt{1 - \gamma_2} - \sqrt{1 - \gamma_1} < 0.$
- $\gamma_2 - \gamma_1 < 0 \rightarrow \gamma_2 < \gamma_1 \rightarrow -\gamma_2 > -\gamma_1 \rightarrow 1 - \gamma_2 > 1 - \gamma_1 \rightarrow \sqrt{1 - \gamma_2} > \sqrt{1 - \gamma_1} \rightarrow \sqrt{1 - \gamma_2} - \sqrt{1 - \gamma_1} > 0.$
- $\gamma_2 - \gamma_1 = 0 \rightarrow \sqrt{1 - \gamma_2} - \sqrt{1 - \gamma_1} = 0.$

From these outcomes, we can tell that  $\gamma_2 - \gamma_1$  and  $\sqrt{1 - \gamma_2} - \sqrt{1 - \gamma_1}$  have a different sign  $\forall \gamma_1, \gamma_2$ . In consequence we can write the sum inside the absolute value of the third term of (5) as

$$(5) = \left| 2|\sqrt{1 - \gamma_2} - \sqrt{1 - \gamma_1}| - |\gamma_2 - \gamma_1| \right|, \quad (6)$$

that is to say, the absolute value of computing the subtraction of each of the original absolute values. To further expand the expression in (6), we use

$$\begin{aligned} |(\sqrt{1 - \gamma_2} - \sqrt{1 - \gamma_1})(\sqrt{1 - \gamma_2} + \sqrt{1 - \gamma_1})| &= |1 - \gamma_2 - 1 + \gamma_1| \\ &= |\gamma_2 - \gamma_1| \rightarrow 2|\sqrt{1 - \gamma_2} - \sqrt{1 - \gamma_1}||\sqrt{1 - \gamma_2} + \sqrt{1 - \gamma_1}| \\ &= 2|\gamma_2 - \gamma_1| \rightarrow 2|\sqrt{1 - \gamma_2} - \sqrt{1 - \gamma_1}| = \frac{2|\gamma_2 - \gamma_1|}{|\sqrt{1 - \gamma_2} + \sqrt{1 - \gamma_1}|} \\ &\rightarrow 2|\sqrt{1 - \gamma_2} - \sqrt{1 - \gamma_1}| \geq |\gamma_2 - \gamma_1|, \end{aligned} \quad (7)$$

$\forall \gamma_1, \gamma_2$  where the last inequality comes from the fact that

- $|\sqrt{1 - \gamma_2} - \sqrt{1 - \gamma_1}| \in (0, 2] \rightarrow 0 < \frac{1}{2}|\sqrt{1 - \gamma_2} - \sqrt{1 - \gamma_1}| \leq 1 \rightarrow \frac{2}{|\sqrt{1 - \gamma_2} + \sqrt{1 - \gamma_1}|} \geq 1$
- $|\sqrt{1 - \gamma_2} - \sqrt{1 - \gamma_1}| = 0 \rightarrow 2|\sqrt{1 - \gamma_2} - \sqrt{1 - \gamma_1}| = |\gamma_2 - \gamma_1| = 0.$

Having shown this result, we can work on (6) even further by removing the absolute value, since we have shown that the subtraction will always be  $\geq 0$ :

$$(6) = 2|\sqrt{1 - \gamma_2} - \sqrt{1 - \gamma_1}| - |\gamma_2 - \gamma_1|. \quad (8)$$

We finish by introducing (8) into expression (5):

$$\begin{aligned} (5) &= \\ &\quad \frac{|\gamma_1 - \gamma_2|}{4} + \frac{|\gamma_1 - \gamma_2|}{4} + \frac{1}{2}|\sqrt{1 - \gamma_2} - \sqrt{1 - \gamma_1}| - \frac{|\gamma_2 - \gamma_1|}{4} \\ &= \frac{1}{4}|\gamma_1 - \gamma_2| + \frac{1}{2}|\sqrt{1 - \gamma_2} - \sqrt{1 - \gamma_1}| \end{aligned} \quad (9)$$

If we now compare (4) and (9), it is clear that both of them are the same, which implies that

$$\|\mathcal{N}_{\text{ADPTA}}(\gamma_1) - \mathcal{N}_{\text{ADPTA}}(\gamma_2)\|_\diamond = \|\mathcal{N}_{\text{ADCTA}}(\gamma_1) - \mathcal{N}_{\text{ADCTA}}(\gamma_2)\|_\diamond, \quad (10)$$

and so concludes the proof for the proposition.  $\square$

## Supplementary Note 2: Additional Numerical analysis

In the main text, numerical simulations of the diamond norm distance were presented in order to assess the difference between the static channel assumption and the proposed time-varying quantum channel model. Here we provide additional numerical analysis that was omitted for clarity in the main text. This data is presented here for completeness purposes.

### Boxplot analysis for $T_1 \approx T_2$ and $T_2$ -dominated scenarios

We provide additional boxplot analysis for the  $T_1 \approx T_2$  and  $T_2$ -dominated superconducting qubit scenarios presented in the main text (see table 2 of the article for more information). Here we provide boxplot analysis for the combined amplitude and phase damping channel, and omit results for their twirl version for simplicity purposes. The results for the twirled approximated channels will be similar.

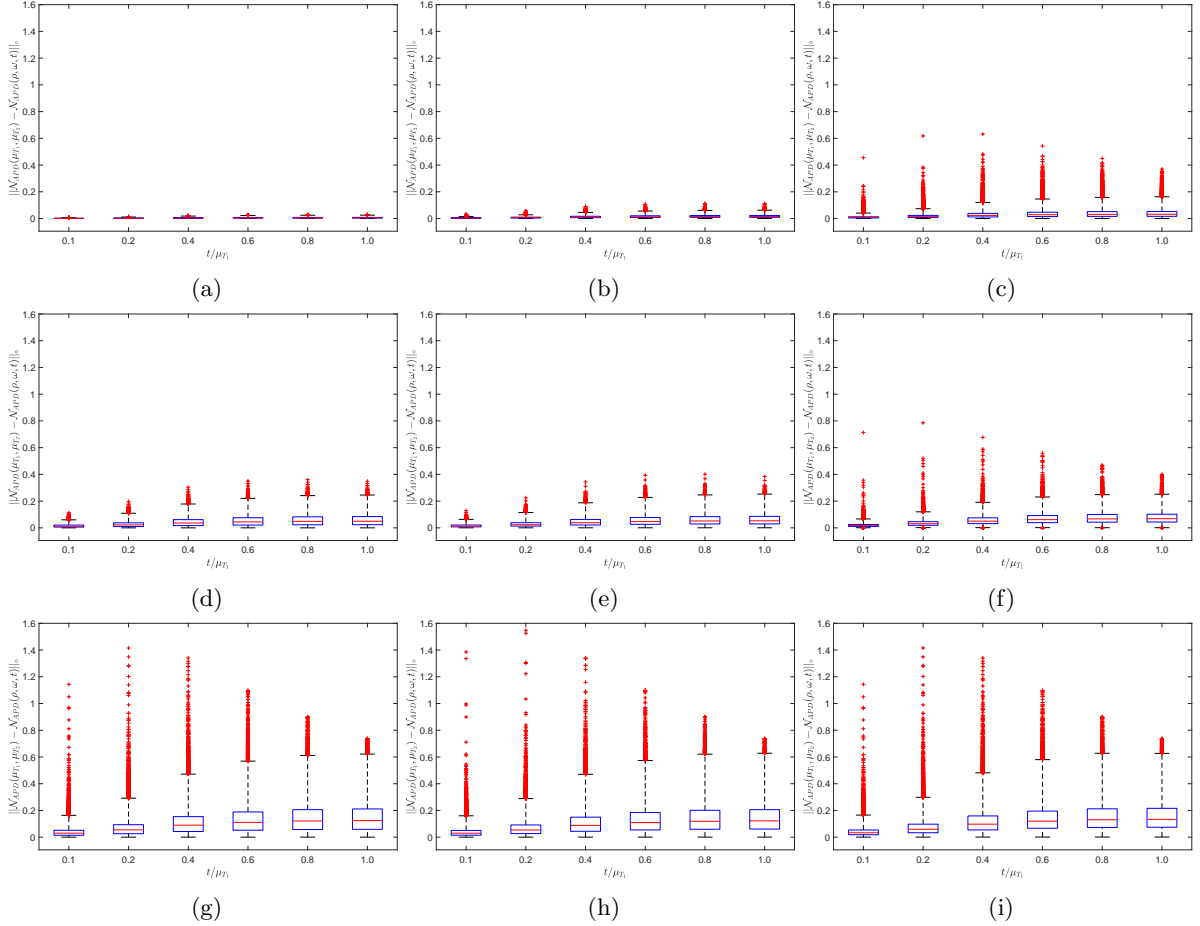

Supplementary Figure 1: **Boxplot representation of the simulations of the diamond norm distance  $\|\mathcal{N}(\mu_{T_1}, \mu_{T_2}) - \mathcal{N}(\rho, \omega, t)\|_\diamond$  for the  $T_1 \approx T_2$  scenario and TVAPD channel (see Table 2 in the main article).** **a**  $c_v(T_1) = 1\%, c_v(T_\phi) = 1\%$ . **b**  $c_v(T_1) = 1\%, c_v(T_\phi) = 10\%$ . **c**  $c_v(T_1) = 1\%, c_v(T_\phi) = 25\%$ . **d**  $c_v(T_1) = 10\%, c_v(T_\phi) = 1\%$ . **e**  $c_v(T_1) = 10\%, c_v(T_\phi) = 10\%$ . **f**  $c_v(T_1) = 10\%, c_v(T_\phi) = 25\%$ . **g**  $c_v(T_1) = 25\%, c_v(T_\phi) = 1\%$ . **h**  $c_v(T_1) = 25\%, c_v(T_\phi) = 10\%$ . **i**  $c_v(T_1) = 25\%, c_v(T_\phi) = 25\%$ . The adjusted boxplots used here are presented in the Methods section. Outlier data is represented with red crosses.

Supplementary Figures 1 and 2 show the boxplot analysis of the diamond norm distance for the  $T_1 \approx T_2$  and  $T_2$ -dominated scenarios studied in the main text considering the combined amplitude and phase damping channel. The trend observed in the main text for  $T_1$ -limited superconducting qubits can also be appreciated in these figures. For both figures, increasing the coefficient of variation of the  $T_1$  and  $T_\phi$  random variables results in a higher spread of the diamond norm distance between the static and TV channels. Consequently, for low variation of the decoherence parameters (see Supplementary Figures 1a, 1b, 2a and 2b), assuming that the channel has a static behaviour is valid. For milder coefficients of variation (see Supplementary Figures 1c, 1d, 1e, 2c, 2d and 2e) the static assumption starts to diverge from the TV channel models, and implications for the QECCs will start to occur. Finally, for the high values of  $c_v(T_1)$  and  $c_v(T_\phi)$  (see Supplementary Figures 1f, 1g, 1h, 1i, 2f, 2g, 2h and 2i), both channel models differ substantially and the non-dynamic assumption is flawed. Note that as discussed in the main text, the variation of the relaxation time has more impact in the channel fluctuations than the variation of the pure dephasing (recall that relaxation is part of the dephasing time  $T_2$ ). Thus, the scenarios with low  $c_v(T_1)$  and notable  $c_v(T_\phi)$  can be considered static (for example, as it can be seen in Supplementary Figures 1b and 2b).

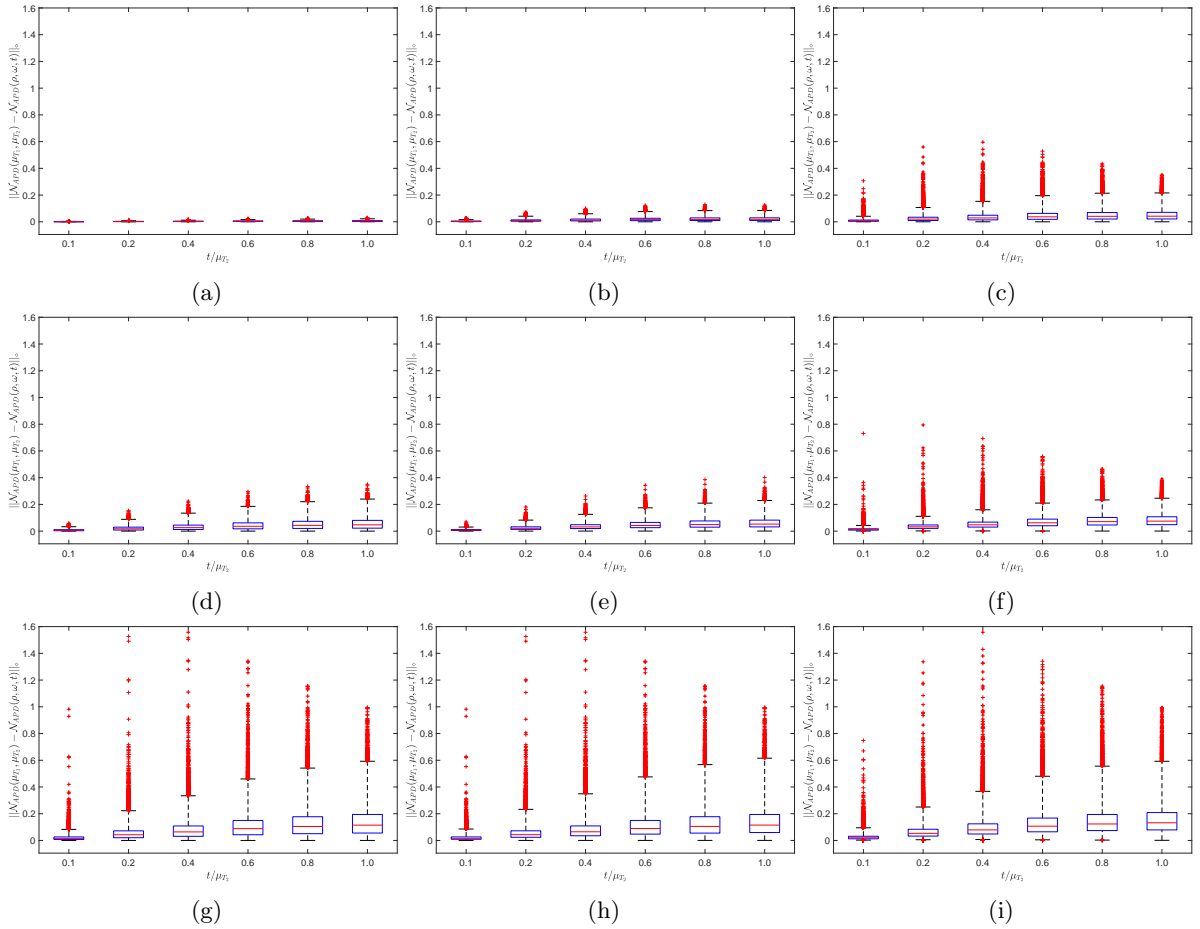

Supplementary Figure 2: **Boxplot representation of the simulations of the diamond norm distance  $\|\mathcal{N}(\mu_{T_1}, \mu_{T_2}) - \mathcal{N}(\rho, \omega, t)\|_\diamond$  for the  $T_2$ -dominated scenario and TVAPD channel (see Table 2 in the main article).** **a**  $c_v(T_1) = 1\%, c_v(T_\phi) = 1\%$ . **b**  $c_v(T_1) = 1\%, c_v(T_\phi) = 10\%$ . **c**  $c_v(T_1) = 1\%, c_v(T_\phi) = 25\%$ . **d**  $c_v(T_1) = 10\%, c_v(T_\phi) = 1\%$ . **e**  $c_v(T_1) = 10\%, c_v(T_\phi) = 10\%$ . **f**  $c_v(T_1) = 10\%, c_v(T_\phi) = 25\%$ . **g**  $c_v(T_1) = 25\%, c_v(T_\phi) = 1\%$ . **h**  $c_v(T_1) = 25\%, c_v(T_\phi) = 10\%$ . **i**  $c_v(T_1) = 25\%, c_v(T_\phi) = 25\%$ . The adjusted boxplots used here are presented in the Methods section. Outlier data is represented with red crosses.

This additional boxplot analysis of the TVAPD channels is useful in order to further confirm the results obtained in the main text. This way, superconducting qubits that present pure dephasing channels that require attention are also affected by the variation of the decoherence parameters. Thus, the TVQC model is relevant for all types of superconducting qubits that present fluctuations of  $T_1$  and  $T_\phi$  with coefficients of variation that are high enough.

## Numerical analysis for the superconducting qubits of [3]

In the article we conducted an extensive numerical analysis in order to study how the fluctuations of the decoherence parameters in superconducting qubits affect the channel models used to describe quantum noise effects. We did so by studying the possible qubit scenarios depending on the weight of the  $T_1$  and  $T_2$  times on the noise, and by varying the “intensity” of the fluctuations (quantified by the coefficient of variation of the random variables that describe the relaxation and pure dephasing times). Here, we provide the same analysis in terms of the mean diamond norm distance and the boxplot depiction of the distribution of the diamond norm distance between the static and TV channels for the specific qubits studied in [3].

As studied in the main text, the superconducting qubits of [3] are  $T_1$ -limited qubits (they reach the limit  $T_2 \approx 2T_1$ ), and, thus, the channel models of interest will be the static and TV amplitude damping channels and their twirled approximations. Supplementary Table 1 presents the mean relaxation time,  $\mu_{T_1}$ , and its standard deviation,  $\sigma_{T_1}$ , for the different superconducting qubit scenarios experimentally studied in [3]. Additionally, we also provide the coefficient of variations for such parameters, which we have used in the main text to quantify how strong the effect of the fluctuations is when comparing the static and the TV channel models.

Supplementary Table 1: Coeffients of variation for the random variables  $T_1(\omega) = T_1(\omega, t)|_{t=0}, \forall t \in [0, T], T \ll T_c$  associated to each of the scenarios in [3] (See Table 1 in the main text). It is common to express the CVs as a percentage.

| Name  | $\mu_{T_1} [\mu\text{s}]$ | $\sigma_{T_1} [\mu\text{s}]$ | $c_v(\%)$ |
|-------|---------------------------|------------------------------|-----------|
| QA_C5 | 44.49                     | 11.7                         | 26.3      |
| QB_C5 | 81.63                     | 17.01                        | 20.84     |
| QA_C6 | 46.64                     | 10.24                        | 21.96     |
| QB_C6 | 71.22                     | 14.31                        | 20.09     |

Supplementary Figure 3 presents the results obtained for the specific experiments in [3] in terms of the mean diamond norm distance. The results here resemble the ones presented in the numerical analysis of the main text. The mean distance in terms of the diamond norm increases with time reaching peak values at around  $t/\mu_{T_1} \approx 1$ . The coefficient of variation captures how different will the static and TV channel models be in average, as a higher  $c_v(T_1)$  implies a higher value of the mean diamond norm distance for all processing times. Consequently, we further corroborate the results obtained via numerical simulation in the main text by studying the specific experiments realized in [3] for superconducting qubits.

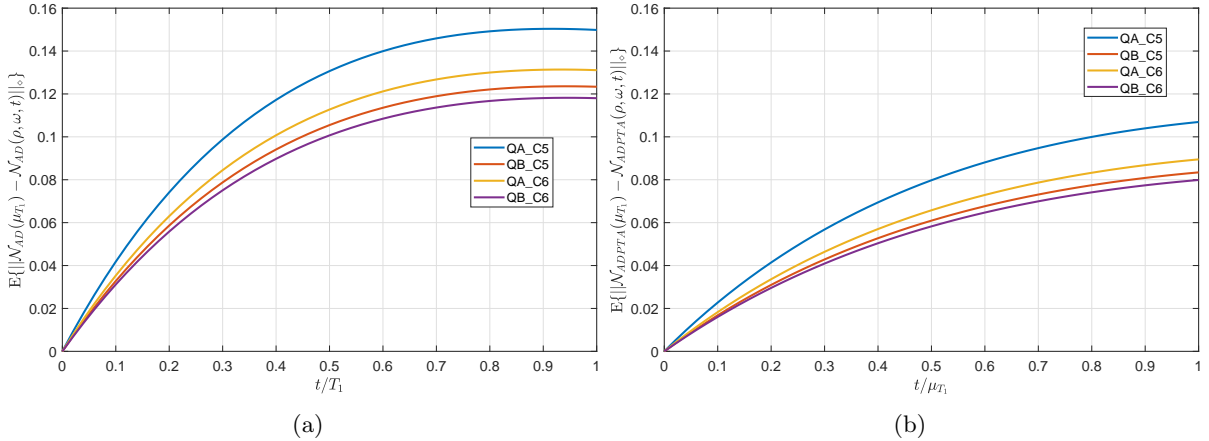

Supplementary Figure 3: **Mean diamond norm distance  $E\{\|\mathcal{N}(\mu_{T_1}) - \mathcal{N}(\rho, \omega, t)\|_\diamond\}$  between the static and the proposed time-varying quantum channels.** The simulation for the calculation is done by using the parameters for the different superconducting qubits and cooldowns from table 1 in the main article. **a**  $T_1$ -limited TVAD. **b**  $T_1$ -limited TVADPTA/TVADCTA. The diamond norm distance between ADPTA and ADCTA channels obtained from AD channels with parameters  $\gamma_1, \gamma_2$  is the same, and thus Supplementary Figure 3b will be the exact same for the mean diamond norm distance of the TVADCTA channels.

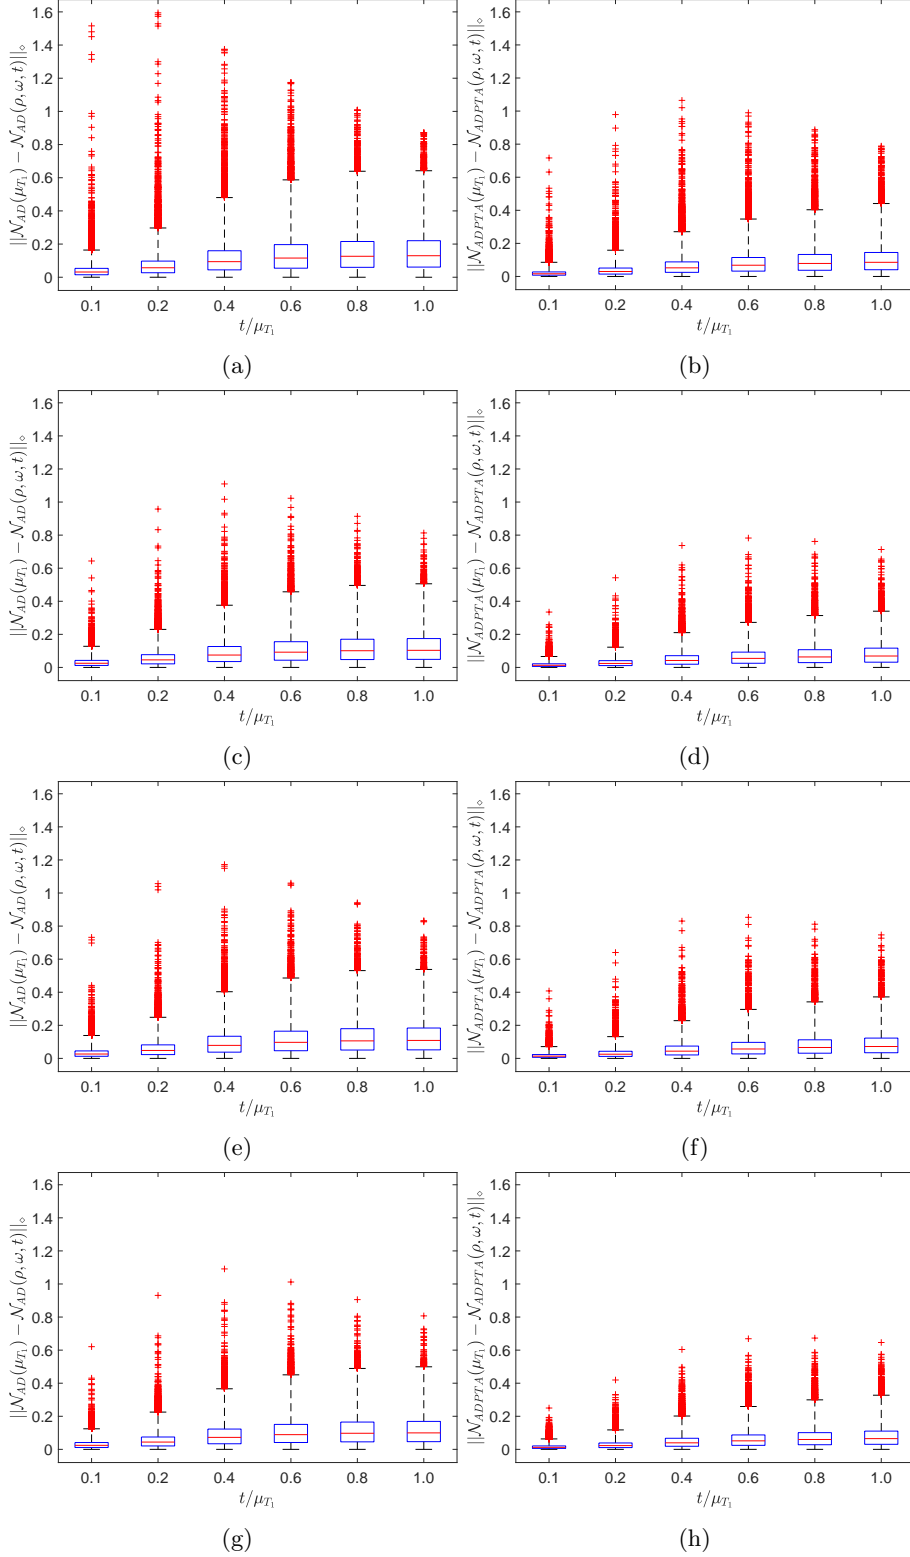

Supplementary Figure 4: **Boxplot representation of the simulations of the diamond norm distance  $\|\mathcal{N}(\mu_{T_1}) - \mathcal{N}(\rho, \omega, t)\|_\diamond$ .** **a** QA\_C5 TVAD. **b** QA\_C5 TVADPTA/TVADCTA. **c** QB\_C5 TVAD. **d** QB\_C5 TVADPTA/TVADCTA. **e** QA\_C6 TVAD. **f** QA\_C6 TVADPTA/TVADCTA. **g** QB\_C6 TVAD. **h** QB\_C6 TVADPTA/TVADCTA. The adjusted boxplots used are presented in the Methods section. Outlier data is represented with red crosses.

Finally, we also study the variability of the diamond norm distance in a similar manner to the numerical analysis, that is, by means of boxplots. Supplementary Figure 4 shows the results obtained

for the qubit scenarios of [3]. These results also corroborate the conclusions reached in the main text. It can be seen that the shape of the boxplots resemble the mean values presented in Supplementary Figure 3, but showing a high spread and a big amount of outlier events. Note that the coefficient of variation is around  $c_v(T_1) \approx [20, 26]\%$  for all the scenarios considered, and, thus, the variability expected is high, similar to the  $c_v(T_1) = 25\%$  case studied in the article. The variability is depicted both for the original amplitude damping channels and for their twirled versions, implying that the consideration of TV channels is relevant for superconducting qubits similar to the ones in [3]. The impact of a higher coefficient of variation is also appreciable here since a higher  $c_v(T_1)$  implies a higher spread. However, due to the closeness of the values of such parameter, all the scenarios present significant fluctuations.

To sum up, we provide a similar analysis to the one presented in the main text, but for the specific dataset of [3]. The conclusions obtained are, as expected, similar to the ones in the article. This further corroborates the need of constructing superconducting qubits (both in terms of construction and cooldown) that not only have long coherence times, but also low fluctuations around its mean value. It also speaks towards the need of studying the limits of QECC and the construction of optimized correction methods for superconducting qubits for whom the TVQC model is relevant (i.e. when the variability of the decoherence parameters around the mean is significant).

## Supplementary References

- [1] Etchezarreta Martinez, J., Fuentes, P., Crespo, P. M., & Garcia-Frías, J. Approximating Decoherence Processes for the Design and Simulation of Quantum Error Correction Codes on Classical Computers. *IEEE Access* **8**, 172623–172643 (2020).
- [2] Benenti, G. & Strini, G. Computing the distance between quantum channels: Usefulness of the Fano representation. *J. Phys. B: At. Mol. Opt. Phys.* **43**, 215508 (2010).
- [3] Burnett, J. J. et al. Decoherence benchmarking of superconducting qubits. *npj Quantum Inf.* **5**, 54 (2019).
